# Supplementary material for: Learning NEAT Emergent Behaviors in Robot Swarms
Source: arXiv:2309.14663 source file (2024-08-08)
Supplement: Supplementary file 1 [file appendixA.tex]

\section*{Appendix A}
\label{appendixA}
\begin{table}[htbp]
\caption{NEAT Parameter Selection}
\begin{center}
\begin{tabular}{|c|c|}
\hline
\multicolumn{2}{|c|}{\textbf{Evolutionary Parameters}} \\
\hline
\textbf{\textit{Parameter}}& \textbf{\textit{Value}}\\
\hline
pop\_size & 300\\
\hline
reset\_on\_extinction & False\\
\hline
no\_fitness\_termination & True\\
\hline
\multicolumn{2}{|c|}{\textbf{Stagnation Parameters}} \\
\hline
\textbf{\textit{Parameter}}& \textbf{\textit{Value}}\\
\hline
species\_fitness\_func & mean\\
\hline
max\_stagnation & 20\\
\hline
species\_elitism & 2\\
\hline
\multicolumn{2}{|c|}{\textbf{Reproduction Parameters}} \\
\hline
\textbf{\textit{Parameter}}& \textbf{\textit{Value}}\\
\hline
elitism & 2\\
\hline
survival\_threshold & 0.2\\
\hline
min\_species\_size & 2\\
\hline
\multicolumn{2}{|c|}{\textbf{Species Parameters}} \\
\hline
\textbf{\textit{Parameter}}& \textbf{\textit{Value}}\\
\hline
compatibility\_threshold & 3.0\\
\hline
\multicolumn{2}{|c|}{\textbf{Genome Parameters}} \\
\hline
\textbf{\textit{Parameter}}& \textbf{\textit{Value}}\\
\hline
activation\_default & sigmoid\\
\hline
activation\_mutate\_rate & 0.0\\
\hline
activation\_options & sigmoid\\
\hline
aggregation\_default & sum\\
\hline
aggregation\_mutate\_rate & 0.0\\
\hline
aggregation\_options & sum\\
\hline
bias\_init\_mean & 0.0\\
\hline
bias\_init\_stdev & 1.0\\
\hline
bias\_init\_type & gaussian\\
\hline
bias\_max\_value & 30.0\\
\hline
bias\_min\_value & -30.0\\
\hline
bias\_mutate\_power & 0.5\\
\hline
bias\_mutate\_rate & 0.7\\
\hline
bias\_replace\_rate & 0.1\\
\hline
compatibility\_disjoint\_coefficient & 1.0\\
\hline
compatibility\_weight\_coefficient & 0.5\\
\hline
conn\_add\_prob & 0.5\\
\hline
conn\_delete\_prob & 0.5\\
\hline
enabled\_default & True\\
\hline
enabled\_mutate\_rate & 0.01\\
\hline
feed\_forward & True\\
\hline
initial\_connection & full\_nodirect\\
\hline
node\_add\_prob & 0.2\\
\hline
node\_delete\_prob & 0.2\\
\hline
num\_hidden & 0\\
\hline
num\_inputs & N/A$^{\mathrm{a}}$\\
\hline
num\_outputs & N/A$^{\mathrm{a}}$\\
\hline
response\_init\_mean & 1.0\\
\hline
response\_init\_stdev & 0.0\\
\hline
response\_init\_type & gaussian\\
\hline
response\_max\_value & 30.0\\
\hline
response\_min\_value & -30.0\\
\hline
response\_mutate\_power & 0.0\\
\hline
response\_mutate\_rate & 0.0\\
\hline
response\_replace\_rate & 0.0\\
\hline
weight\_init\_mean & 0.0\\
\hline
weight\_init\_stdev & 1.0\\
\hline
weight\_init\_type & gaussian\\
\hline
weight\_max\_value & 30\\
\hline
weight\_min\_value & -30\\
\hline
weight\_mutate\_power & 0.5\\
\hline
weight\_mutate\_rate & 0.8\\
\hline
weight\_replace\_rate & 0.1\\
\hline
\multicolumn{2}{l}{$^{\mathrm{a}}$: Dependant on the experiment.}
\end{tabular}
\label{neat_table}
\end{center}
\end{table}

In \tabref{neat_table}, we list the parameters we use for NEAT training. In this section we explain the reason for our choice of a few of them. The description of each parameters function can be found in the NEAT documentation \cite{neat_docs}.
\begin{itemize}
    \item Evolutionary Parameters

    We choose a pop\_size of 300 since the NEAT examples have around this as a population size
    \item Stagnation Parameters

    species\_fitness\_func decides how species are evaluated based on their members. More fit species are better able to reproduce, and less fit species are more likely to go extinct.
    
    We choose mean as species\_fitness\_func to reduce the impact of a lucky trial on species fitness. We want our evolved species to consistently achieve high fitness as opposed to using risky behaviors and having a few members get lucky.
    
    \item Reproduction Parameters:

    We choose an elitism parameter of 2 since we want to be sure at least 2 genomes are left in each genome to be able to reproduce. For the same reason, we choose a min\_species\_size of 2, so that after each reproduction, there are at least 2 genomes in each species.
    \item Species Parameters:

    compatibility\_threshold is a measure of how far apart two genomes must be before they are considered from different species. The genome distance is calculated using the parameters compatibility\_disjoint\_coefficient and compatibility\_weight\_coefficient. For all three of these, we use the values found in NEAT examples.
    \item Genome Parameters:

    We use the values from NEAT example experiments for the parameters describing the initialization and mutation of network nodes, weights, and connections.

    The num\_inputs and num\_outputs vary based on the experiment run.
    
\end{itemize}
